# Supplementary material for: Adaptive Coordination Offsets for Signalized Arterial Intersections using Deep Reinforcement Learning
Source: arXiv:2008.02691 source file (2022-08-29)
Supplement: Supplementary file 1 [file appendices.tex]

\appendices

\section*{Schedule of offset configurations}
\begin{table}[ht]
\caption{SYNCHRO Offsets in (a) AM and (b) Noon (c) PM scenarios}
\centering
\resizebox{\columnwidth}{!}{%
\begin{tabular}[width=\columnwidth]{c c c c c c} 
\hline\hline 
\toprule
Time              & Offset 1 & Offset 2 & Offset 3 & Offset 4 & Offset 5 \\ \midrule
5:00 AM - 5:45 AM & 75       & 66       & 14       & 19       & 48       \\ \midrule
5:45 AM - 6:30 AM & 40       & 40       & 5        & 0        & 5        \\ \midrule
6:30 AM - 9:00 AM & 60       & 60       & 65       & 75       & 5        \\ \midrule
9:00AM - 11:00 AM & 40       & 40       & 5        & 0        & 5        \\  \bottomrule
\hline
\hline
\end{tabular}
}
\resizebox{\columnwidth}{!}{%
\begin{tabular}[width=\columnwidth]{c c c c c c} 
\hline\hline 
\toprule
Time                & Offset 1 & Offset 2 & Offset 3 & Offset 4 & Offset 5 \\ \midrule
10:00 AM - 12:00 NN & 40       & 40       & 5        & 0        & 5        \\ \midrule
12:00 NN - 2:00 PM  & 0        & 0        & 55       & 55       & 55       \\ \bottomrule
\hline
\hline
\end{tabular}
}
\resizebox{\columnwidth}{!}{%
\begin{tabular}[width=\columnwidth]{c c c c c c} 
\hline\hline 
\toprule
Time              & Offset 1 & Offset 2 & Offset 3 & Offset 4 & Offset 5 \\ \midrule
2:00 PM - 4:00 PM & 0        & 0        & 55       & 55       & 55       \\ \midrule
4:00 PM - 7:00 PM & 60       & 60       & 65       & 75       & 5        \\ \midrule
7:00 PM - 8:30 PM & 0        & 0        & 55       & 55       & 55       \\ \midrule
8:30 PM - 9:00 PM & 40       & 40       & 5        & 0        & 5        \\ \bottomrule
\hline 
\end{tabular}
}
\label{table:sychoffsets_am} 
\end{table}

\begin{table}[ht]
\caption{Deep RL Offsets in (a) AM and (b) Noon and (c) PM scenarios}
\centering
\resizebox{\columnwidth}{!}{%
\begin{tabular}[width=\columnwidth]{c c c c c c} 
\hline\hline 
\toprule
Time                & Offset 1 & Offset 2 & Offset 3 & Offset 4 & Offset 5 \\ \midrule
5:00 AM - 6:00 AM   & 31       & 8        & 60       & 43       & 6        \\ \midrule
6:00 AM - 8:00 AM   & 31       & 55       & 60       & 43       & 6        \\ \midrule
8:00 AM - 8:15 AM   & 70       & 86       & 82       & 43       & 107      \\ \midrule
8:15 AM - 8:30 AM   & 70       & 86       & 82       & 59       & 107      \\ \midrule
8:30 AM - 8:45 AM   & 37       & 73       & 82       & 59       & 107      \\ \midrule
8:45 AM - 9:15 AM   & 37       & 86       & 82       & 59       & 107      \\ \midrule
9:15 AM - 10:45 AM  & 37       & 73       & 82       & 59       & 107      \\ \midrule
10:45 AM - 11:00 AM & 70       & 86       & 82       & 59       & 107      \\ \bottomrule
\hline
\hline
\end{tabular}
}
\resizebox{\columnwidth}{!}{%
\begin{tabular}[width=\columnwidth]{c c c c c c} 
\hline\hline 
\toprule
Time                & Offset 1 & Offset 2 & Offset 3 & Offset 4 & Offset 5 \\ \midrule
10:00 AM - 11:45 AM & 70       & 86       & 82       & 59       & 107      \\ \midrule
11:45 AM - 12:00 NN & 37       & 72       & 60       & 43       & 107      \\ \midrule
12:00 NN - 12:45 PM & 31       & 55       & 60       & 43       & 6        \\ \midrule
12:45 PM - 1:00 PM  & 31       & 55       & 60       & 71       & 6        \\ \midrule
1:00 PM - 1:15 PM   & 37       & 73       & 82       & 59       & 107      \\ \midrule
1:15 PM - 1:30 PM   & 71       & 72       & 60       & 97       & 48       \\ \midrule
1:30 PM - 1:45 PM   & 71       & 72       & 88       & 97       & 48       \\ \midrule
1:45 PM - 2:00 PM   & 31       & 72       & 60       & 43       & 6        \\ \bottomrule
\hline
\hline
\end{tabular}
}

\resizebox{\columnwidth}{!}{%
\begin{tabular}[width=\columnwidth]{c c c c c c} 
\hline
\hline 
Time              & Offset 1 & Offset 2 & Offset 3 & Offset 4 & Offset 5 \\ \midrule
2:00 PM - 2:30 PM & 50       & 55       & 15       & 43       & 81       \\ \midrule
2:30 PM - 2:45 PM & 71       & 72       & 60       & 43       & 48       \\ \midrule
2:45 PM - 3:00 PM & 31       & 55       & 60       & 43       & 6        \\ \midrule
3:00 PM - 3:30 PM & 71       & 72       & 88       & 97       & 48       \\ \midrule
3:30 PM - 3:45 PM & 31       & 55       & 60       & 43       & 6        \\ \midrule
3:45 PM - 4:15 PM & 71       & 72       & 60       & 97       & 48       \\ \midrule
4:15 PM - 4:30 PM & 31       & 72       & 60       & 43       & 6        \\ \midrule
4:30 PM - 4:45 PM & 31       & 55       & 60       & 97       & 6        \\ \midrule
4:45 PM - 5:15 PM & 31       & 55       & 60       & 43       & 6        \\ \midrule
5:15 PM - 5:30 PM & 71       & 72       & 60       & 97       & 6        \\ \midrule
5:30 PM - 7:45 PM & 31       & 55       & 60       & 43       & 6        \\ \midrule
7:45 PM - 8:00 PM & 71       & 72       & 88       & 97       & 46       \\ \midrule
8:00 PM - 8:45 PM & 31       & 55       & 60       & 43       & 6        \\ \midrule
8:45 PM - 9:00 PM & 19       & 104      & 60       & 72       & 107      \\ \bottomrule
\hline 
\end{tabular}
}
\label{table:sychoffsets_noon_pm} 
\end{table}
